# Supplementary material for: Synthetic Quorum Sensing and Absorbing Phase Transitions in Colloidal Active Matter
Source: arXiv:2502.13919 ancillary file (2025-10-07)
Supplement: Supplementary file 1 [file SM_v3.pdf]

# Supplemental Material for: Quorum sensing and absorbing phase transitions in colloidal active matter

Thibault Lefranc\*

*ENSL, CNRS, Laboratoire de physique, Université de Lyon, F-69342 Lyon, France*

Alberto Dinelli\*

*Department of Biochemistry, University of Geneva, 1211 Geneva, Switzerland and  
Université Paris Cité, MSC, UMR 7057 CNRS, 75013 Paris, France*

Carla Fernandez Rico

*Department of Materials, ETH Zürich, 8093 Zürich, Switzerland*

Roel P. A. Dullens

*Institute for Molecules and Materials, Radboud University Heyendaalseweg 135, 6525 AJ Nijmegen, The Netherlands*

Julien Tailleur†

*Department of Physics, Massachusetts Institute of Technology, Cambridge, Massachusetts 02139, USA*

Denis Bartolo†

*ENSL, CNRS, Laboratoire de physique, Université de Lyon, F-69342 Lyon, France*

(Dated: December 17, 2024)

## CONTENTS

|                                                                                     |    |
|-------------------------------------------------------------------------------------|----|
| I. Coarse-graining of rod dynamics with density-dependent rates                     | 3  |
| II. Mean-field dynamics of homogeneous systems                                      | 4  |
| A. Weakly-arresting regime ( $\alpha_0 < \beta_0$ ).                                | 5  |
| B. Strongly-arresting regime ( $\alpha_0 > \beta_0$ ).                              | 6  |
| III. Coarse-graining in the presence of density-dependent rates and pairwise forces | 6  |
| IV. Local approximation and effective-equilibrium theory                            | 8  |
| V. Generalized thermodynamics of active rods                                        | 10 |
| A. Active pressure in the active liquid phase                                       | 10 |
| B. Direct pressure in the active liquid phase                                       | 11 |
| C. Direct pressure in the arrested phase                                            | 11 |
| D. Direct pressure in a well-mixed system                                           | 12 |
| E. Numerical tests                                                                  | 13 |
| F. From the generalized pressure to the binodal densities                           | 13 |
| VI. Mechanical pressure in Quincke rods                                             | 13 |
| VII. Numerical details                                                              | 16 |
| A. Figure parameters                                                                | 16 |
| B. Bulk pressure measurements                                                       | 16 |
| C. Pressure measurements in the presence of a wall                                  | 17 |
| D. Coarsening                                                                       | 17 |
| E. Area fraction                                                                    | 17 |
| F. Binodals                                                                         | 18 |

---

\* These authors contributed equally to this work.

† Corresponding authors. Email: denis.bartolo@ens-lyon.fr and jgt@mit.edu

## G. Hysteresis

18

## VIII. Captions for Supplementary Movies

18

## References

19

The Supplemental Material contains detailed theoretical derivations of our results together with their numerical validations.

In Sec. I we derive the coarse-grained dynamics of rods with density-dependent rates in the absence of pairwise forces, Eq. (4) of the main text. Sec. II is then devoted to the study of the corresponding mean-field relaxation dynamics, Eq. (3) of the main text. In Sec. III we extend the coarse-graining procedure to a system of rolling and standing ABPs with both quorum-sensing rates and pairwise forces, Eq. (6) of the main text. Starting from the hydrodynamics Eq. (6), in Sec. IV we then build the effective-equilibrium theory, Eq. (7) of the main text. To provide quantitative predictions for the phase-separation binodals we need to determine a closed formula for the effective free-energy  $\mathcal{G}$  appearing in Eq. (7) of the main text. This is derived in Sec. V, where we provide closed expressions for the contributions to the bulk pressure in each phase and use them to build the free-energy density  $g(\rho)$ . Next, to elucidate the results of Fig. 6b of the main text, we conclude this theoretical part with a detailed discussion on how bulk and wall pressures are related in the liquid and arrested phases, Sec. VI.

We then provide details on the numerical protocols we employed. These are reported in Sec. VII, together with the parameter list for the figures of the main text. Finally, in Sec. VIII we provide the captions for the Supplementary Movies.

## I. COARSE-GRAINING OF ROD DYNAMICS WITH DENSITY-DEPENDENT RATES

In this section, we derive the coarse-grained dynamics of active Brownian rods with transition rates between the rolling and standing states that depend on the local density of particles, Eq. (4) of the main text, starting from their microscopic dynamics. For particles in the rolling ( $R$ ) and standing ( $S$ ) states, the dynamics respectively read:

$$R: \quad \dot{\mathbf{r}}_i = v_0 \mathbf{u}_i(\theta_i), \quad \dot{\theta}_i = \sqrt{2D_r} \eta_i(t), \quad (S1)$$

$$S: \quad \dot{\mathbf{r}}_i = 0, \quad (S2)$$

where  $\mathbf{r}_i$  and  $\mathbf{u}_i = (\cos \theta_i, \sin \theta_i)$  denote the position and orientation vectors of particle  $i$ , respectively, and  $\eta_i(t)$  is a Gaussian white noise with unit variance and zero mean. Particles switch between the two states with a ‘standing rate’  $\alpha$  and a ‘rolling rate’  $\beta$ , as defined in Eqs. (1)–(2) of the main text. To account for how interactions between the rods induce these transitions, we take the rates  $\alpha$  and  $\beta$  to be functions of the effective densities  $\tilde{\rho}(\mathbf{r}) \equiv K * \rho(\mathbf{r})$  and  $\tilde{\rho}_R(\mathbf{r}) \equiv K * \rho_R(\mathbf{r})$ , respectively, where  $*$  denotes a convolution and  $K(\mathbf{r})$  is a normalized isotropic bell-shaped kernel (See App. B1 in the main text). The support of  $K$  is a disc of radius  $\ell_r$ , so that the density fields are sampled within a finite interaction range that represents the length of the rods.

Let us first introduce some useful notations. The fluctuating density of particles in the standing state is denoted  $\hat{\rho}_S(\mathbf{r})$  and defined as:

$$\hat{\rho}_S(\mathbf{r}) = \sum_{i=1}^N \delta(\mathbf{r} - \mathbf{r}_i(t)) \delta_{s_i, S}, \quad (S3)$$

where  $s_i$  specifies the state of particle  $i$ . We use a hat to denote a fluctuating function  $\hat{f}$  and we denote its noise-average as  $f \equiv \langle \hat{f} \rangle$ .

Particles in the rolling state are characterized both by their positions and their orientations. We denote their fluctuating density in  $(\mathbf{r}, \theta)$  space by  $\hat{\psi}_R$ , defined by:

$$\hat{\psi}_R(\mathbf{r}, \theta; t) = \sum_{i=1}^N \delta(\mathbf{r} - \mathbf{r}_i(t)) \delta(\theta - \theta_i(t)) \delta_{s_i, R}. \quad (S4)$$

The successive moments of  $\hat{\psi}_R$  allows us to define the spatial density, polar and nematic fields as:

$$\hat{\rho}_R(\mathbf{r}, t) = \int d\theta \hat{\psi}_R, \quad (S5)$$

$$\hat{\mathbf{m}}_R(\mathbf{r}, t) = \int d\theta \hat{\psi}_R \mathbf{u}, \quad (S6)$$

$$\hat{\mathbf{Q}}_R(\mathbf{r}, t) = \int d\theta \hat{\psi}_R \left( \mathbf{u} \otimes \mathbf{u} - \frac{\mathbf{I}}{2} \right). \quad (S7)$$

Finally, the total particle density field is defined as:  $\hat{\rho}(\mathbf{r}, t) = \hat{\rho}_S + \hat{\rho}_R$ .

To derive the mean-field hydrodynamics of  $\rho = \langle \hat{\rho} \rangle$ , we first consider separately the standing and rolling particles. At mean-field level, the time evolution of  $\rho_S$  reads:

$$\partial_t \rho_S = \alpha(\tilde{\rho}) \rho_S - \beta(\tilde{\rho}_R) \rho_S, \quad (S8)$$

while the (Ginzburg-Landau) mean-field dynamics of  $\psi_R(\mathbf{r}, \theta, t)$  reads

$$\partial_t \psi_R = -\nabla_{\mathbf{r}} \cdot [v_0 \mathbf{u} \psi_R] + \nabla_{\theta}^2 [D_r \psi_R] - \alpha(\tilde{\rho}) \psi_R + \frac{\beta(\tilde{\rho}_R)}{2\pi} \rho_S. \quad (S9)$$

Integrating Eq. (S9) over  $\theta$ , we obtain the dynamics of  $\rho_R(\mathbf{r})$  as:

$$\partial_t \rho_R = -\nabla_{\mathbf{r}} \cdot [v_0 \mathbf{m}_R] - \alpha(\tilde{\rho}) \rho_R(\mathbf{r}) + \beta(\tilde{\rho}_R) \rho_S(\mathbf{r}), \quad (S10)$$

so that the evolution of the total density  $\rho(\mathbf{r})$  reads:

$$\partial_t \rho = -\nabla_{\mathbf{r}} \cdot [v_0 \mathbf{m}_R]. \quad (S11)$$

Let us now show how to express  $\mathbf{m}_R$  in terms of  $\rho$  and  $\rho_R$ . Projecting Eq. (S9) onto the first and second harmonics

of  $\psi$  as in Eqs. (S6)–(S7), we obtain the evolution equations of the average polar and nematic fields:

$$\partial_t \mathbf{m}_R = -\nabla_{\mathbf{r}} \cdot \left[ v_0 \left( \mathbf{Q}_R + \frac{\mathbf{I}}{2} \rho_R \right) \right] - (D_r + \alpha) \mathbf{m}_R \quad (\text{S12})$$

$$\partial_t \mathbf{Q}_R = -\nabla_{\mathbf{r}} \cdot \left[ v_0 \left( \langle \mathbf{u}^{\otimes 3}, \psi_R \rangle + \frac{\mathbf{I}}{2} \otimes \mathbf{m} \right) \right] - (4D_r + \alpha) \mathbf{Q}_R, \quad (\text{S13})$$

where  $\langle \mathbf{S}, \psi_R \rangle \equiv \int d\mathbf{u} \mathbf{S} \psi_R$  denotes the integration over the unit sphere.

We note that  $\mathbf{m}_R$  and  $\mathbf{Q}_R$ —as all the harmonics of  $\psi_R$ —undergo fast relaxations with finite decay times. On the contrary, the conserved density field  $\rho$  is a slow mode—the only one in the system—whose relaxation time diverges with the system size. On such macroscopic time scales, we can thus set  $\dot{\mathbf{m}}_R = \dot{\mathbf{Q}}_R = 0$  in Eqs. (S12)–(S13). For the same reason, the time-derivative of the fast density modes,  $\partial_t \rho_R$  and  $\partial_t \rho_S$ , can be set to zero in Eqs. (S8), (S10). To leading order in the gradients of the density field  $\rho(\mathbf{r})$ , we then find[1]:

$$\partial_t \mathbf{Q}_R(\mathbf{r}) = 0 \quad \Rightarrow \quad \mathbf{Q}_R(\mathbf{r}) = \mathcal{O}(\nabla_{\mathbf{r}} \rho), \quad (\text{S14})$$

$$\partial_t \mathbf{m}_R(\mathbf{r}) = 0 \quad \Rightarrow \quad \mathbf{m}_R(\mathbf{r}) \simeq -\frac{v_0}{2[\alpha(\rho) + D_r]} \nabla_{\mathbf{r}} \rho_R, \quad (\text{S15})$$

$$\partial_t \rho_S = 0 \quad \Rightarrow \quad \rho_S(\mathbf{r}) \simeq \frac{\alpha(\rho)}{\beta(\rho_R)} (\rho - \rho_S), \quad (\text{S16})$$

$$\partial_t \rho_R = 0 \quad \Rightarrow \quad \rho_R(\mathbf{r}) \simeq \rho - \rho_S. \quad (\text{S17})$$

All fast modes are thus enslaved to the slow density field  $\rho(\mathbf{r})$ . Finally, we can rewrite Eq. (S11) as

$$\partial_t \rho = -\nabla_{\mathbf{r}} \cdot \mathbf{J}, \quad \text{with} \quad \mathbf{J} = -\mathcal{D}_{\text{eff}} \nabla_{\mathbf{r}} \rho_R(\rho) \quad \text{and} \quad \mathcal{D}_{\text{eff}} = \frac{v_0^2}{2[D_r + \alpha(\rho)]}, \quad (\text{S18})$$

which corresponds to Eq. (4) of the main text.

To get more insight into dynamics (S18), we rewrite it as:

$$\partial_t \rho = \nabla_{\mathbf{r}} \cdot [M(\mathbf{r}) \nabla_{\mathbf{r}} \mathbf{u}(\rho_R)] , \quad \mathbf{u}(\rho_R) \equiv \log \rho_R, \quad M(\mathbf{r}, [\tilde{\rho}, \rho_R]) \equiv \frac{v_0^2 \rho_R}{2[D_r + \alpha(\rho)]}, \quad (\text{S19})$$

where  $M$  is a collective mobility while  $\mathbf{u}(\rho_R)$  plays the role of an effective chemical potential. The latter is clearly entropic in nature, since  $\mathbf{u}(\rho_R) = \frac{d}{d\rho_R} [\rho_R (\ln \rho_R - 1)]$ : the dynamics is driven by the diffusion of rolling particles and tends to spread them uniformly in space. Note that the collective mobility  $M$  is proportional to the local number of rolling particles, so that it vanishes in their absence.

## II. MEAN-FIELD DYNAMICS OF HOMOGENEOUS SYSTEMS

In this section we consider the evolution of uniform profiles in the  $(\rho_S, \rho_R)$  space, given by Eq. (3) of the main text:

$$\dot{\rho}_R = \beta(\rho_R) \rho_S - \alpha(\rho_0) \rho_R \quad \text{and} \quad \dot{\rho}_S = -\dot{\rho}_R. \quad (\text{S20})$$

We derive analytically the fixed points of the relaxation dynamics, together with their basins of attraction, for the standing and rolling rates given by:

$$R \xrightarrow{\alpha} S, \quad \alpha(\rho) = \alpha_0 (\rho - \bar{\rho}) \Theta(\rho - \bar{\rho}) \quad (\text{S21})$$

$$S \xrightarrow{\beta} R, \quad \beta(\rho_R) = \beta_0 \rho_R, \quad (\text{S22})$$

corresponding to Eqs. (1)–(2) of the main text. Depending on whether  $\alpha_0$  is greater or smaller than  $\beta_0$ , there are two possible scenarios for the relaxation dynamics, depicted in Fig. 1, which we now detail.

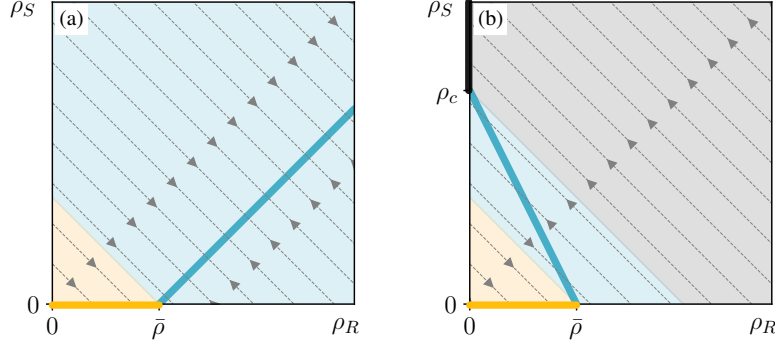

SI FIG. 1. Mean-field streamplots. Dashed lines represent streamlines, and are parametrized by the total density  $\rho_0$  through  $\rho_S + \rho_R = \rho_0$ . Solid lines represent stable attractors. (a) Weakly-arresting regime  $\alpha_0 < \beta_0$ . For  $\rho_0 < \bar{\rho}$  the active liquid (ochre) is the only stable attractor, while at  $\rho_0 > \bar{\rho}$  we observe a well-mixed phase with finite densities of standing and rolling rods (teal). (b) Strongly-arresting regime  $\alpha_0 > \beta_0$ . For  $\rho_0 < \bar{\rho}$  the active liquid (ochre) is still the only stable attractor. At intermediate densities  $\bar{\rho} < \rho_0 < \rho_c$  we observe a well-mixed fixed point (teal); At large densities  $\rho_0 \geq \rho_c$  the arrested phase is the only attractor (black).

### A. Weakly-arresting regime ( $\alpha_0 < \beta_0$ ).

The mean-field dynamics in the ‘weakly-arresting regime’, when  $\alpha_0 < \beta_0$ , is illustrated in Fig. 1a. First, we note that the fully arrested solution  $\rho_R \equiv 0$  is always an unstable fixed point. To see this, we linearize Eq. (S20) around  $(\rho_R^*, \rho_S^*) \equiv (0, \rho_0)$ . Defining  $\delta\rho_R \equiv \rho_R - \rho_R^*$ , and using the fact that mass conservation imposes  $\delta\rho_R = -\delta\rho_S$ , the linearized dynamics of  $\delta\rho_R$  reads:

$$\begin{aligned} \delta\dot{\rho}_R(t) &= -\alpha_0(\rho_0 - \bar{\rho})\Theta(\rho_0 - \bar{\rho})\delta\rho_R + \beta_0\delta\rho_R\rho_0 \\ &= [\beta_0\rho_0 + \alpha_0(\rho_0 - \bar{\rho})\Theta(\rho_0 - \bar{\rho})]\rho_0\delta\rho_R. \end{aligned} \quad (\text{S23})$$

In Eq. (S23), the growth rate of  $\delta\rho_R$  is positive for all  $\rho_0$  and the arrested fixed point is always unstable.

We now study the other fixed points of the mean-field dynamics. For each of them, we determine their basin of attraction by studying the fully non-linear dynamics.

- At small densities, when  $\rho_0 < \bar{\rho}$ , Eq. (S20) is solved by  $(\rho_R^*, \rho_S^*) = (\rho_0, 0)$ , which corresponds to an active liquid phase. In this regime, the dynamics (S20) reduces to:

$$\begin{pmatrix} \dot{\rho}_R \\ \dot{\rho}_S \end{pmatrix} = \begin{pmatrix} \beta_0\rho_R\rho_S \\ -\beta_0\rho_R\rho_S \end{pmatrix}, \quad (\text{S24})$$

so that  $\dot{\rho}_R > 0$  everywhere. Since  $\rho_R \leq \rho_0$ , the active fixed point  $(\rho_R^*, \rho_S^*) = (\rho_0, 0)$  is a non-linear attractor when  $\rho_0 < \bar{\rho}$ .

- For  $\rho_0 > \bar{\rho}$ , Eq. (S20) admits a well-mixed fixed point  $(\rho_R^*, \rho_S^*)$ , with both rolling and standing particles whose densities are respectively given by:

$$\begin{aligned} \rho_R^* &= \left(1 - \frac{\alpha_0}{\beta_0}\right)\rho_0 + \frac{\alpha_0}{\beta_0}\bar{\rho}, \\ \rho_S^* &= \frac{\alpha_0}{\beta_0}\rho_0 - \frac{\alpha_0}{\beta_0}\bar{\rho}. \end{aligned} \quad (\text{S25})$$

Defining  $\delta\rho_{R,S} \equiv \rho_{R,S} - \rho_{R,S}^*$ , the dynamics (S20) becomes:

$$\begin{pmatrix} \delta\dot{\rho}_R \\ \delta\dot{\rho}_S \end{pmatrix} = \kappa(\delta\rho_R) \begin{pmatrix} \delta\rho_R \\ \delta\rho_S \end{pmatrix} \quad (\text{S26})$$

with  $\kappa(\delta\rho_R) = -\beta_0\delta\rho_R + [3\alpha_0(\rho_0 - \bar{\rho}) - \beta_0\bar{\rho}]$ . For all admissible values of  $\delta\rho_R$ , i.e. such that  $0 \leq \rho_R \leq \rho_0$ ,  $\kappa(\delta\rho_R) < 0$  and perturbations are suppressed: the non-trivial fixed point is a stable attractor for the non-linear dynamics. Note that the well-mixed phase extends up to infinite values of  $\rho_0$ .

The weakly-arresting regime thus does not allow for a stable arrested phase. This is inconsistent with our experimental results and, in the main text, we thus focus on the strongly-arresting regime that we now describe.

### B. Strongly-arresting regime ( $\alpha_0 > \beta_0$ ).

The dynamics of the ‘strongly-arresting regime’, when  $\alpha_0 > \beta_0$ , is described in Fig. 1b. There are three different regimes.

- At small densities, when  $\rho_0 < \bar{\rho}$ , the sole stable fixed point is the active one,  $(\rho_0, 0)$ . This fixed point is a non-linear attractor in this region, as the dynamics can be recast in the form of Eq. (S24), analogously to the weakly-arresting case.
- Upon increasing the density, when  $\rho_0 > \bar{\rho}$ , we find again a well-mixed stable fixed point (S25). However, since  $\alpha_0 > \beta_0$ ,  $\rho_R^*(\rho_0)$  decreases with  $\rho_0$  and the well-mixed fixed point disappears at a critical density  $\rho_c \equiv \bar{\rho}/(1 - \beta_0/\alpha_0)$ , which is computed by setting  $\rho_R^* = 0$  in Eq. (S25). In this intermediate region,  $\bar{\rho} < \rho_0 < \rho_c$ , Eq. (S26) still holds,  $\kappa < 0$ , and the well-mixed fixed point is the only stable attractor.
- Beyond the critical density, when  $\rho_0 > \rho_c$ , the arrested phase  $(\rho_R^*, \rho_S^*) = (0, \rho_0)$  becomes the only stable attractor. Defining  $\delta\rho_{R,S} = \rho_{R,S} - \rho_{R,S}^*$ , the dynamics in this region can be rewritten as:

$$\begin{pmatrix} \delta\dot{\rho}_R \\ \delta\dot{\rho}_S \end{pmatrix} = \gamma(\delta\rho_R) \begin{pmatrix} \delta\rho_R \\ \delta\rho_S \end{pmatrix} \quad (\text{S27})$$

with  $\gamma(\delta\rho_R) = -[\alpha_0(\rho_0 - \bar{\rho}) + \beta_0(\rho_0 - \delta\rho_R)]$ . Since  $0 < \delta\rho_R < \rho_0$ ,  $\gamma$  is always negative and the arrested fixed point with  $\rho_R = 0$  is the sole stable attractor.

Finally, note that, for any value of  $\rho_0$ , there is a unique stable fixed point. The line of stable fixed points can thus be parametrized by  $\rho_0$  and hence, when we refer to such fixed points, we write  $(\rho_R(\rho_0), \rho_S(\rho_0))$ .

### III. COARSE-GRAINING IN THE PRESENCE OF DENSITY-DEPENDENT RATES AND PAIRWISE FORCES

In this section we derive the expression of the coarse-grained particle current given in Eq. (6) of the main text, which holds in the presence of both quorum sensing and pairwise forces. To proceed, we start from the microscopic dynamics given in Eq. (5) of the main text. Using the notation introduced in Eqs. (S3)-(S7), we have:

$$\begin{aligned} \partial_t \rho_S &= -\nabla_{\mathbf{r}} \cdot \left[ \mu \left\langle \sum_{j=1}^N \mathbf{f}(|\mathbf{r} - \mathbf{r}_j|) \hat{\rho}_S(\mathbf{r}) \right\rangle \right] + \alpha(\bar{\rho})\rho_R - \beta(\bar{\rho}_R)\rho_S \\ &= -\nabla_{\mathbf{r}} \cdot \left[ \mu \left\langle \int d^2\mathbf{r}' \mathbf{f}(|\mathbf{r} - \mathbf{r}'|) \hat{\rho}(\mathbf{r}') \hat{\rho}_S(\mathbf{r}) \right\rangle \right] + \alpha(\bar{\rho})\rho_R - \beta(\bar{\rho}_R)\rho_S, \end{aligned} \quad (\text{S28})$$

$$\partial_t \psi_R = -\nabla_{\mathbf{r}} \cdot \left[ v_0 \mathbf{u} \psi_R + \mu \left\langle \int d^2\mathbf{r}' \mathbf{f}(|\mathbf{r} - \mathbf{r}'|) \hat{\rho}(\mathbf{r}') \hat{\psi}_R(\mathbf{r}) \right\rangle \right] + \nabla_{\theta}^2 [D_r \psi_R] - \alpha \psi_R + \frac{\beta \rho_S}{2\pi}, \quad (\text{S29})$$

$$\partial_t \rho_R = -\nabla_{\mathbf{r}} \cdot \left[ v_0 \mathbf{m}_R + \mu \left\langle \int d^2\mathbf{r}' \mathbf{f}(|\mathbf{r} - \mathbf{r}'|) \hat{\rho}(\mathbf{r}') \hat{\rho}_R(\mathbf{r}) \right\rangle \right] - \alpha \rho_R(\mathbf{r}) + \beta \rho_S(\mathbf{r}), \quad (\text{S30})$$

so that, using  $\rho = \rho_R + \rho_S$  and summing Eqs (S28) and (S30), the evolution of  $\rho$  reads:

$$\partial_t \rho = -\nabla \cdot \mathbf{J} = -\nabla_{\mathbf{r}} \cdot \left[ v_0 \mathbf{m}_R + \mu \left\langle \int d^2\mathbf{r}' \mathbf{f}(|\mathbf{r} - \mathbf{r}'|) \hat{\rho}(\mathbf{r}') \hat{\rho}(\mathbf{r}) \right\rangle \right]. \quad (\text{S31})$$

In Eq. (S31), the particle current comprises an active term,  $v_0 \mathbf{m}_R$ , and a contribution stemming from the pairwise forces. To close the hydrodynamics (S31), we compute the dynamics of the higher-order harmonics of  $\psi_R$  as:

$$\partial_t \mathbf{m}_R = -\nabla_{\mathbf{r}} \cdot \left[ v_0 \left( \mathbf{Q}_R + \frac{\mathbf{I}}{2} \rho_R \right) + \mu \left\langle \int d^2 \mathbf{r}' \mathbf{f}(|\mathbf{r} - \mathbf{r}'|) \hat{\rho}(\mathbf{r}') \hat{\mathbf{m}}_R(\mathbf{r}) \right\rangle \right] - (D_r + \alpha) \mathbf{m}_R, \quad (\text{S32})$$

$$\begin{aligned} \partial_t \mathbf{Q}_R = & -\nabla_{\mathbf{r}} \cdot \left[ v_0 \left( \langle \mathbf{u}^{\otimes 3}, \psi_R \rangle + \frac{\mathbf{I}}{2} \otimes \mathbf{m} \right) + \mu \left\langle \int d^2 \mathbf{r}' \mathbf{f}(|\mathbf{r} - \mathbf{r}'|) \hat{\rho}(\mathbf{r}') \hat{\mathbf{Q}}_R(\mathbf{r}) \right\rangle \right] \\ & - (4D_r + \alpha) \mathbf{Q}_R, \end{aligned} \quad (\text{S33})$$

where  $\langle \mathbf{S}, \psi_R \rangle \equiv \int d\mathbf{u} \mathbf{S} \psi_R$  denotes the integration of  $\mathbf{S} \psi_R$  over the unit sphere.

The fast relaxation of non-conserved fields allows us to set  $\dot{\mathbf{m}}_R = 0$ ,  $\dot{\mathbf{Q}}_R = 0$ ,  $\dot{\rho}_S = \dot{\rho}_R = 0$ . The polar field  $\mathbf{m}_R$  thus relaxes to:

$$\begin{aligned} \mathbf{m}_R = & -\frac{1}{D_r + \alpha} \nabla_{\mathbf{r}} \cdot \left[ v_0 \left( \frac{\rho_R}{2} \mathbf{I} + \mathbf{Q}_R \right) + \mu \mathcal{I}_m \right], \\ \text{where } \mathcal{I}_{m,\alpha\beta}(\mathbf{r}) \equiv & \int d^2 \mathbf{r}' f_\alpha(|\mathbf{r} - \mathbf{r}'|) \langle \hat{\rho}(\mathbf{r}') m_{R,\beta}(\mathbf{r}) \rangle. \end{aligned} \quad (\text{S34})$$

Using this expression in Eq. (S31) yields:

$$\partial_t \rho = -\nabla_{\mathbf{r}} \cdot \mathbf{J}, \quad (\text{S35})$$

$$\mathbf{J} = -\frac{v_0}{D_r + \alpha(\tilde{\rho})} \nabla_{\mathbf{r}} \cdot \left[ v_0 \left( \frac{\rho_R}{2} \mathbf{I} + \mathbf{Q}_R \right) + \mu \mathcal{I}_m \right] + \mu \left\langle \int d^2 \mathbf{r}' \mathbf{f}(|\mathbf{r} - \mathbf{r}'|) \hat{\rho}(\mathbf{r}') \hat{\rho}(\mathbf{r}) \right\rangle. \quad (\text{S36})$$

We first note that the last term in Eq. (S36) can be written as the divergence of an Irving-Kirkwood stress tensor [2]:  $\mu \langle \int d^2 \mathbf{r}' \mathbf{f}(\mathbf{r} - \mathbf{r}') \hat{\rho}(\mathbf{r}') \hat{\rho}(\mathbf{r}) \rangle = \mu \nabla_{\mathbf{r}} \cdot \boldsymbol{\sigma}_{\text{IK}}$ . After some algebra, this allows us to rewrite the particle current as the sum of the divergence of a stress tensor and of an additional term:

$$\mathbf{J} = \mu \nabla_{\mathbf{r}} \cdot \left( -\frac{v_0^2 \rho_R}{2\mu[D_r + \alpha(\tilde{\rho})]} \mathbf{I} - \frac{v_0^2}{\mu[D_r + \alpha(\tilde{\rho})]} \mathbf{Q}_R - \frac{v_0 \mathcal{I}_m}{D_r + \alpha(\tilde{\rho})} + \boldsymbol{\sigma}_{\text{IK}} \right) + \mu \boldsymbol{\Delta}(\mathbf{r}), \quad (\text{S37})$$

where  $\boldsymbol{\Delta}(\mathbf{r})$  reads:

$$\boldsymbol{\Delta}(\mathbf{r}) \equiv \left[ \frac{v_0^2}{\mu} \left( \frac{\rho_R}{2} \mathbf{I} + \mathbf{Q}_R \right) + v_0 \mathcal{I}_m \right] \cdot \nabla_{\mathbf{r}} \left[ \frac{1}{D_r + \alpha(\tilde{\rho})} \right]. \quad (\text{S38})$$

Identifying the active stress tensor as:

$$\boldsymbol{\sigma}_a \equiv -\frac{v_0}{\mu[D_r + \alpha(\tilde{\rho})]} \left( \frac{v_0 \rho_R}{2} \mathbf{I} + v_0 \mathbf{Q}_R + \mu \mathcal{I}_m \right), \quad (\text{S39})$$

we recast the current into

$$\mathbf{J} = \mu \nabla_{\mathbf{r}} \cdot \boldsymbol{\sigma}_a + \mu \nabla_{\mathbf{r}} \cdot \boldsymbol{\sigma}_{\text{IK}} + \mu \boldsymbol{\Delta}, \quad (\text{S40})$$

which corresponds to Eq. (6) of the main text.

We now conclude by discussing the physical meaning of the terms in Eq. (S40). The active stress tensor generalizes the standard expression for PFAPs [3, 4] to a system of active particles with switching rates. On the one hand, the presence of a stopping rate  $\alpha(\tilde{\rho})$  renormalizes the mass of the polar field  $D_r \rightarrow D_r + \alpha(\tilde{\rho})$ ; on the other hand, since the active stress results exclusively from the dynamics of rolling particles, the usual terms in  $\rho, \mathbf{Q}$  are replaced by  $\rho_R, \mathbf{Q}_R$ , respectively. Having introduced the active stress tensor, the term  $\boldsymbol{\Delta}(\mathbf{r})$  can be re-expressed as:

$$\boldsymbol{\Delta}(\mathbf{r}) = \frac{1}{D_r + \alpha(\tilde{\rho})} \boldsymbol{\sigma}_a(\mathbf{r}) \cdot \nabla_{\mathbf{r}} \alpha(\tilde{\rho}) = \frac{\alpha'(\tilde{\rho})}{D_r + \alpha(\tilde{\rho})} \boldsymbol{\sigma}_a(\mathbf{r}) \cdot \nabla_{\mathbf{r}} \tilde{\rho}. \quad (\text{S41})$$

We thus conclude that  $\boldsymbol{\Delta}$  vanishes both in the liquid phase, where  $\alpha' \equiv 0$ , and in the arrested one, where  $\boldsymbol{\sigma}_a \equiv 0$ . Subsequently, we expect this term to provide only an interfacial contribution in phase-separated configurations.

All in all, by defining the total stress tensor  $\boldsymbol{\sigma} \equiv \boldsymbol{\sigma}_a + \boldsymbol{\sigma}_{\text{IK}}$ , we see that, in the steady state,  $\mathbf{J} = 0$  and mechanical

balance reads:

$$\nabla_{\mathbf{r}} \cdot \boldsymbol{\sigma} = -\Delta(\mathbf{r}) . \quad (\text{S42})$$

#### IV. LOCAL APPROXIMATION AND EFFECTIVE-EQUILIBRIUM THEORY

In this section we derive the effective-equilibrium theory Eq. (7) of the main text, starting from the hydrodynamics (S40). The idea is to retain only the leading-order terms in a gradient expansion, which are expected to govern the dynamics of long-wavelength modes. The corresponding approximations are standard and are expected to work qualitatively, but fail quantitatively when the interfaces between coexisting phases are sharp [4]. For clarity, we discuss them below:

1. We assume that  $\tilde{\rho} \approx \rho$ , corresponding to a truncation to leading order of

$$\begin{aligned} \int d\mathbf{r}' K(\mathbf{r}') \rho(\mathbf{r} - \mathbf{r}') &\simeq \int d\mathbf{r}' K(\mathbf{r}') [\rho(\mathbf{r}) - \mathbf{r}' \cdot \nabla \rho(\mathbf{r}) + \frac{1}{2} (\mathbf{r}')^2 \Delta \rho(\mathbf{r})] \\ &\simeq \rho(\mathbf{r}) \int d\mathbf{r}' K(\mathbf{r}') = \rho(\mathbf{r}) \end{aligned} \quad (\text{S43})$$

Accordingly, the transition rates  $\alpha(\cdot)$  and  $\beta(\cdot)$  become local functions of the density fields  $\rho$  and  $\rho_R$  respectively.

2. We neglect the gradient terms in the dynamics of  $\rho_S$  and  $\rho_R$ , given by Eqs. (S28), (S30). By discarding these transport terms we retain only the relaxation part given by Eq. (3) of the main text.
3. We assume that fast density modes  $(\rho_R, \rho_S)$  relax instantaneously to the corresponding fixed point of Eq. (3) of the main text.  $\rho_R$  and  $\rho_S$  thus become enslaved to the total density  $\rho$ .
4. We neglect all higher-order contributions in gradients to the active stress tensor  $\boldsymbol{\sigma}_a$  in Eq. (S39).

- First, we show that the nematic field  $\mathbf{Q}_R \sim \mathcal{O}(\nabla_{\mathbf{r}})$  provides a subleading contribution compared to  $\rho_R \mathbf{I} \sim \mathcal{O}(1)$ . To see this, we use the fact that  $\mathbf{Q}$  is a fast mode to set  $\partial_t \mathbf{Q}_R = 0$  in Eq. (S7), so that:

$$\mathbf{Q}_R = -\frac{1}{D_r + \alpha} \nabla_{\mathbf{r}} \cdot \left[ v_0 \left( \langle \mathbf{u}^{\otimes 3}, \psi_R \rangle + \frac{\mathbf{I}}{2} \otimes \mathbf{m} \right) + \mu \left\langle \int d^2 \mathbf{r}' \mathbf{f}(|\mathbf{r} - \mathbf{r}'|) \hat{\rho}(\mathbf{r}') \hat{\mathbf{Q}}_R(\mathbf{r}) \right\rangle \right] = \mathcal{O}(\nabla_{\mathbf{r}}) .$$

- Then, we turn to the tensor  $\mathcal{I}_m$ . At leading order in gradients, we write this contribution as:

$$\mathcal{I}_m \equiv \left\langle \int d^2 \mathbf{r}' \mathbf{f}(|\mathbf{r} - \mathbf{r}'|) \hat{\rho}(\mathbf{r}') \hat{\mathbf{m}}_R(\mathbf{r}) \right\rangle = \frac{\rho_R \mathbf{I}}{2\mu} [v(\rho) - v_0] + \mathcal{O}(\nabla_{\mathbf{r}}) . \quad (\text{S44})$$

where we introduced an effective speed  $v(\rho)$  that we derive below, and which results from the pairwise forces between the particles.

To derive Eq. (S44), we first consider a homogeneous and isotropic system with average densities  $(\rho_R, \rho_S)$  and total conserved density  $\rho$ . Due to isotropy, the correlation in Eq. (S44) is proportional to the identity matrix  $\mathbf{I}$ . The  $xx$ -component of this object, which we denote by  $\mathcal{I}_m$ , can be written explicitly using the definitions (S5), (S6) of  $\hat{\rho}$  and  $\hat{\mathbf{m}}_R$ :

$$\mathcal{I}_m = \left\langle \sum_i \sum_{j \in R} \int d^2 \mathbf{r}' f_x(\mathbf{r} - \mathbf{r}') \delta(\mathbf{r}' - \mathbf{r}_i) \delta(\mathbf{r} - \mathbf{r}_j) \cos(\theta_j) \right\rangle . \quad (\text{S45})$$

In a homogeneous system we can integrate Eq. (S45) over  $\mathbf{r}$  and divide by the total volume  $L_x L_y$ :

$$\mathcal{I}_m = \frac{1}{L_x L_y} \left\langle \sum_i \sum_{j \in R} \int d^2 \mathbf{r} \int d^2 \mathbf{r}' f_x(\mathbf{r} - \mathbf{r}') \delta(\mathbf{r}' - \mathbf{r}_i) \delta(\mathbf{r} - \mathbf{r}_j) \cos(\theta_j) \right\rangle \quad (\text{S46})$$

$$= \frac{1}{L_x L_y} \left\langle \sum_i \sum_{j \in R} f_x(\mathbf{r}_j - \mathbf{r}_i) \cos(\theta_j) \right\rangle . \quad (\text{S47})$$



Since the system is isotropic, we use  $\langle f_x \cos(\theta) \rangle = \langle f_y \sin(\theta) \rangle$  to write:

$$\mathcal{I}_m = \frac{1}{L_x L_y} \left\langle \frac{1}{2} \sum_i \sum_{j \in R} \mathbf{f}(\mathbf{r}_j - \mathbf{r}_i) \cdot \mathbf{u}_j \right\rangle = \frac{1}{L_x L_y} \left\langle \frac{1}{2} \sum_{j \in R} \mathbf{F}_j \cdot \mathbf{u}_j \right\rangle, \quad (\text{S48})$$

where  $\mathbf{F}_j$  is the sum of all pairwise forces acting on  $j$ . By looking at the dynamics of the rolling particle  $j$ , we have that  $\mu \mathbf{F}_j = \dot{\mathbf{r}}_j - v_0 \mathbf{u}_j$ , so:

$$\mathcal{I}_m = \frac{1}{L_x L_y} \frac{1}{2\mu} \left[ \sum_{j \in R} \langle \dot{\mathbf{r}}_j \cdot \mathbf{u}_j \rangle - v_0 \sum_{j \in R} \langle \mathbf{u}_j^2 \rangle \right] = \frac{\rho_R}{2\mu} [\langle \dot{\mathbf{r}} \cdot \mathbf{u} \rangle_R - v_0]. \quad (\text{S49})$$

In the last passage, we used that  $\mathbf{u}^2 = 1$  and homogeneity to express  $\frac{1}{L_x L_y} \sum_{j \in R} = \rho_R \langle \cdot \rangle_R$ , where we introduced the average over rolling particles  $\langle \cdot \rangle_R$ . Finally, we define:

$$v(\rho) \equiv \langle \dot{\mathbf{r}} \cdot \mathbf{u} \rangle_R \quad (\text{S50})$$

as the effective speed of rolling particles along their orientation  $\mathbf{u}$ . We have thus derived Eq. (S44) for a homogeneous system. In the presence of interfaces and density gradients, Eq. (S44) is a leading-order approximation in a gradient expansion.

At this stage, we have a formal expression for  $\mathcal{I}_m$ , but still lack a closed form for  $v(\rho)$ . Motivated by standard results in the literature of PFAPs [3, 5] we take:

$$v(\rho) = v_0 \left( 1 - \frac{\rho}{\rho_J} \right) \Theta(\rho_J - \rho), \quad (\text{S51})$$

where  $\rho_J$  is a free parameter of the model, representing the jamming density for our system.

In conclusion, to leading order in gradients the active stress tensor reads:

$$\boldsymbol{\sigma}_a = -\mathbf{I} \frac{v_0 v(\rho)}{2\mu [D_r + \alpha(\rho)]} \rho_R + \mathcal{O}(\nabla_{\mathbf{r}}), \quad (\text{S52})$$

so that the active pressure  $P_A = -\sigma_{a,xx}$  is given by:

$$\boxed{P_{\text{act}} \approx \frac{v_0 v(\rho)}{2\mu [D_r + \alpha(\rho)]} \rho_R(\rho), \quad v(\rho) = v_0 \left( 1 - \frac{\rho}{\rho_J} \right) \Theta(\rho_J - \rho)} \quad (\text{S53})$$

5. We assume that the Irving-Kirkwood stress tensor  $\boldsymbol{\sigma}_{\text{IK}}$  is isotropic. While this is true in the bulk of both phases, this approximation is expected to fail close to interfaces, where the role of higher-order gradient terms becomes important. Under this approximation, we thus express:

$$\boldsymbol{\sigma}_{\text{IK}} = -P_{\text{dir}}(\rho) \mathbf{I} + \mathcal{O}(\nabla_{\mathbf{r}}), \quad (\text{S54})$$

where  $P_{\text{dir}}$  is the direct pressure.

6. Finally, we neglect all higher-order contributions in gradients in the expression (S41) of  $\boldsymbol{\Delta}$ , which yields:

$$\boldsymbol{\Delta}(\mathbf{r}) = -\frac{\alpha'(\rho)}{D_r + \alpha(\rho)} P_{\text{act}}(\rho) \nabla_{\mathbf{r}} \rho + \mathcal{O}(\nabla_{\mathbf{r}}^2) = -\nabla_{\mathbf{r}} \int^{\rho(\mathbf{r})} \frac{\alpha'(s)}{D_r + \alpha(s)} P_{\text{act}}(s) ds + \mathcal{O}(\nabla_{\mathbf{r}}^2). \quad (\text{S55})$$

In conclusion, within the local approximation we express the particle current  $\mathbf{J}$  as:

$$\mathbf{J} = \mu \nabla_{\mathbf{r}} \cdot \boldsymbol{\sigma} + \mu \boldsymbol{\Delta}(\mathbf{r}) \approx -\mu \nabla_{\mathbf{r}} \tilde{P}(\rho), \quad (\text{S56})$$

where we have introduced the generalized pressure  $\tilde{P}(\rho)$ :

$$\boxed{\tilde{P}(\rho) = \underbrace{P_{\text{dir}}(\rho) + P_{\text{act}}(\rho)}_{P(\rho)} + \int^{\rho} \frac{\alpha'(s)}{D_r + \alpha(s)} P_{\text{act}}(s) ds} . \quad (\text{S57})$$

As we discuss in Sec. VI,  $\tilde{P}$  is not the mechanical pressure of the system, *i.e.* the force density that would be measured by a pressure gauge. Nevertheless, it can be used to build an effective free energy  $\mathcal{G}$  for our system. Indeed, since  $P(\mathbf{r})$  is a local function of  $\rho(\mathbf{r})$ , we can define a generalized free energy density  $g(\rho)$  through:

$$\tilde{P}(\rho) = -g(\rho) + \rho g'(\rho) , \quad \mathcal{G}[\rho] = \int d\mathbf{r} g(\rho(\mathbf{r})) , \quad (\text{S58})$$

so that our dynamics for  $\rho$  becomes a gradient-descent in the  $\mathcal{G}$ -landscape:

$$\partial_t \rho(\mathbf{r}, t) = \nabla_{\mathbf{r}} \cdot \left[ \mu \rho \nabla_{\mathbf{r}} \frac{\delta \mathcal{G}}{\delta \rho(\mathbf{r}, t)} \right] . \quad (\text{S59})$$

We have thus obtained Eq. (7) of the main text. In conclusion, the generalized free-energy density  $g(\rho)$  can be obtained by integrating Eq. (S58), which yields:

$$g(\rho) = \rho \int^{\rho} \frac{\tilde{P}(s)}{s^2} ds . \quad (\text{S60})$$

Applying the common-tangent construction on  $g(\rho)$  we finally obtain the value of the coexisting binodals. To do that we need to find a close expression for  $\tilde{P}(\rho)$ . This is the aim of the next section.

## V. GENERALIZED THERMODYNAMICS OF ACTIVE RODS

In this section, we provide a closed form for the effective free energy  $g(\rho)$  that we use to predict the binodals reported in Fig. 6 of the main text. To do so, we first derive a closed expression for the generalized pressure  $\tilde{P}(\rho)$ , defined in Eq. (S57). At this stage, we are missing:

1. The value of the jamming density  $\rho_J$  in  $v(\rho)$ , see Eq. (S51);
2. A closed expression for the direct pressure  $P_{\text{dir}}(\rho)$  for our system of rolling and standing particles.

We start by discussing how we obtain the value of  $\rho_J$ . For the direct pressure  $P_{\text{dir}}$ , we proceed in three steps: we first provide an expression for  $P_{\text{dir}}$  in the presence of rolling particles, then for standing particles, and finally for a well-mixed system comprising both rolling and standing particles.

### A. Active pressure in the active liquid phase

The active pressure Eq. (S53) is reminiscent of the active pressure in active Brownian particles interacting via pairwise forces (PFAPs) [3]. Indeed, in the active liquid phase where  $\alpha(\rho) = 0$ ,  $\rho_R \equiv \rho$  and the two expressions coincide:

$$P_{\text{act}}^{\text{PFAP}} = \frac{v_0 v(\rho)}{2\mu D_r} \rho , \quad v(\rho) = v_0 \left( 1 - \frac{\rho}{\rho_J} \right) \Theta(\rho_J - \rho) . \quad (\text{S61})$$

For our choice of the particle size  $\sigma = 1$ , we thus determine  $\rho_J$  by fitting the active pressure  $P_{\text{act}}^{\text{PFAP}}(\rho)$  for a system of PFAPs in the absence of  $S \leftrightarrow R$  transitions. We work in the same parameter regime as in the main text:  $v_0 = 10$ ,  $D_r = 2$ ,  $E_0 = 1$ , and obtain a jamming density of  $\rho_J = 1.11 \pm 0.01$  from the fit, see SI Fig. 2a.

In the following, it will be convenient to work with the jamming packing fraction, denoted by  $\eta_J$ , rather than with the corresponding density. The former is defined as:

$$\eta_J = \rho_J \frac{\pi \sigma^2}{4} \quad \text{constant} \quad \Rightarrow \quad \rho_J = \frac{4\eta_J}{\pi} \frac{1}{\sigma^2} . \quad (\text{S62})$$

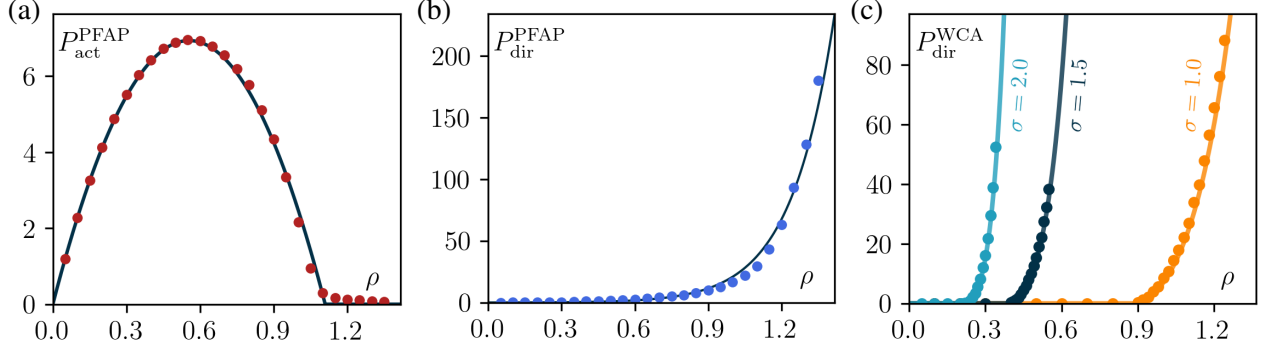

SI FIG. 2. **Fits for the free parameters of the pressure  $\eta_J, \xi, z$  and test for the WCA pressure.** (a) Measurements of the active pressure of PFAPs as a function of the density. The solid line corresponds to the fit obtained via Eq. (S61). (b) Measurement of the direct pressure of PFAPs as a function of the density. The solid line corresponds to the fit obtained via Eq. (S61). (c) Direct pressure in a passive athermal WCA crystal: comparison between simulations and theory from Eq. (S74). The theoretical curves fall on top of the numerical data, validating our prediction. Parameters for panels a,b:  $v_0 = 10, D_r = 2, \sigma = 1, \mu = 1, E_0 = 1$ . Parameters for panel c:  $E_0 = 1$ . In all simulations, the system size is  $200 \times 200$ .

The jamming packing fraction corresponding to our fitted value of  $\rho_J$  is  $\eta_J = 0.872 \pm 0.007$ .

### B. Direct pressure in the active liquid phase

The direct pressure in the liquid phase is equivalent to the direct pressure in PFAPs, which we denote by  $P_{\text{dir}}^{\text{PFAP}}$ . It can be expressed in a scaling form [5, 6]:

$$P_{\text{dir}}^{\text{PFAP}}(\rho) \sim \frac{v_0 \sigma}{\mu} \rho \mathcal{S}[\eta(\rho)] , \quad \eta(\rho) \equiv \rho \frac{\pi \sigma^2}{4} , \quad (\text{S63})$$

where  $\eta$  is the packing fraction associated with  $\rho$ , and  $\mathcal{S}(\cdot)$  an increasing function. Following Ref. [5] we take:

$$\mathcal{S}(\rho) = \exp\left(\xi \frac{\eta}{\eta_J}\right) \quad \Rightarrow \quad \boxed{P_{\text{dir}}^{\text{PFAP}} = z \frac{v_0 \sigma}{\mu} \rho \exp\left(\xi \frac{\eta}{\eta_J}\right)} \quad (\text{S64})$$

where  $z$  and  $\xi$  are free parameters, while  $\eta_J$  is the jamming packing fraction at which  $v(\rho) = 0$ . To determine the values of  $z$  and  $\xi$ , in SI Fig. 2b we fit the direct pressure  $P_d^{\text{PFAP}}$  in simulations of PFAPs as a function of  $\rho$ . The values of the parameters estimated from the fits are  $\eta_J = 0.87$ ,  $z = 0.015$ ,  $\xi = 5.5$ . In the following, we use these values to model the active contribution to the direct pressure.

### C. Direct pressure in the arrested phase

The arrested phase is a system of athermal, passive particles, which arrange in a crystalline configuration at large packing fractions. In this phase, each particle is represented by a circular disc with diameter  $\sigma$ , lying on one vertex of a triangular lattice with spacing  $a$ . To determine the direct pressure in this system, which we denote by  $P_{\text{dir}}^{\text{WCA}}$ , we compute the variation of the total potential energy under an infinitesimal, isotropic compression of the lattice.

Since the interaction potential has a finite cutoff radius  $r_0$ , particles do not interact when  $a > r_0$ , so that the corresponding Irving-Kirkwood pressure is zero. Then, when the system becomes sufficiently packed ( $a < r_0$ ), the pressure in the solid  $P_{\text{dir}}^{\text{WCA}}(a)$  can be defined via the infinitesimal work associated with the isotropic compression of the solid. Let  $\mathcal{A}(a)$  be the total area of a triangular lattice with spacing  $a$  and  $N$  vertices. Then:

$$P_{\text{dir}}^{\text{WCA}}(a) d\mathcal{A} = -dW_{\text{ext}} = dU_{\text{tot}} , \quad (\text{S65})$$

where  $dW_{\text{ext}}$  is the infinitesimal work exerted on the lattice, and  $dU_{\text{tot}}$  the corresponding variation of the lattice

potential energy. Simple geometrical arguments give  $\mathcal{A}(a) = N \frac{a^2 \sqrt{3}}{2}$ , so that:

$$P_{\text{dir}}^{\text{WCA}}(a) = \frac{1}{\sqrt{3}aN} \frac{dU_{\text{tot}}(a)}{da} . \quad (\text{S66})$$

We now have to compute the term  $dU_{\text{tot}}/da$ . In fact,  $U_{\text{tot}}$  is the sum of the potential energies of each bond; each particle interacts with 6 neighbours, and each bond is shared between 2 particles. All in all:

$$\frac{dU_{\text{tot}}}{da} = \frac{6N}{2} \frac{dU_{\text{bond}}}{da} = 3N \frac{dU_{\text{bond}}}{da} , \quad (\text{S67})$$

where  $U_{\text{bond}}$  is the interaction energy of a single bond, which in our case corresponds to the WCA potential energy:

$$U_{\text{bond}}(r) = E_0 \left[ 4 \left( \frac{\sigma^{12}}{r^{12}} - \frac{\sigma^6}{r^6} \right) + 1 \right] \Theta(r_0 - r) . \quad (\text{S68})$$

In conclusion:

$$P_{\text{dir}}^{\text{WCA}}(a) = \frac{\sqrt{3}}{a} \frac{dU_{\text{bond}}}{da} . \quad (\text{S69})$$

For WCA:

$$P_{\text{dir}}^{\text{WCA}}(a) = \frac{24\sqrt{3}}{a^2} E_0 \left( \frac{\sigma}{a} \right)^6 \left[ 2 \left( \frac{\sigma}{a} \right)^6 - 1 \right] \Theta(r_0 - a) , \quad (\text{S70})$$

where the Heaviside function enforces that the pressure is zero at low packing fractions.

Our ultimate goal is to express  $P_{\text{dir}}^{\text{WCA}}$  as a function of the density  $\rho$ . To do that, we first determine the relation between lattice spacing  $a$  and  $\rho$ . Each triangular cell has an area of  $\mathcal{A}_t = a^2 \sqrt{3}/4$ . In a lattice with  $N$  vertices, each vertex belongs to 6 triangles. The total number of triangular cells is then  $6N/3 = 2N$ , where we divide by 3 since each triangle is shared by three vertices. The density of particles in the lattice is then equal to:

$$\rho(a) = \frac{N}{2N\mathcal{A}_t} = \frac{2}{\sqrt{3}a^2} . \quad (\text{S71})$$

The corresponding packing fraction is defined as:

$$\eta(\rho) \equiv \rho(a) \frac{\pi}{4} \sigma^2 , \quad (\text{S72})$$

so that, at the WCA cutoff radius  $r_0 = 2^{1/6}\sigma$ , the critical packing fraction is:

$$\eta_c \equiv \rho(r_0) \frac{\pi}{4} \sigma^2 = \frac{\pi}{2^{4/3}\sqrt{3}} \approx 0.72 . \quad (\text{S73})$$

Eqs. (S71)–(S72) finally allows us to express the pressure  $P_{\text{D}}^{\text{WCA}}$  in Eq. (S70) as:

$$\boxed{P_{\text{dir}}^{\text{WCA}}(\rho) = w E_0 \rho \eta^3 (\eta^3 - \eta_c^3) \Theta(\eta - \eta_c) , \quad \eta_c \equiv \frac{\pi}{2^{4/3}\sqrt{3}} , \quad w \equiv \frac{3^5 2^9}{\pi^6} \approx 129 .} \quad (\text{S74})$$

To confirm whether our computation is correct, we test our theory in numerical simulations of athermal particles at different packing fractions  $\eta$  and sizes  $\sigma$ . As shown in SI Fig. 2c, our theory is in excellent agreement with numerical simulations.

#### D. Direct pressure in a well-mixed system

To obtain a closed expression for the direct pressure as a function of the densities  $P_{\text{dir}}(\rho_R, \rho_S)$  we finally consider a well-mixed homogeneous system containing both standing (S) and rolling (R) particles. As an ansatz for  $P_{\text{dir}}$  we take a combination of the direct pressure in the liquid phase, Eq. (S64), and the direct pressure in the arrested crystal,

Eq. (S74). We propose:

$$P_{\text{dir}}(\rho_R, \rho_S) = P_{\text{dir}}^{(R)} + P_{\text{dir}}^{(S)} \quad (\text{S75})$$

$$\text{where } P_{\text{dir}}^{(R)} = z \frac{v_0 \sigma}{\mu} \rho_R \exp\left(\xi \frac{\eta}{\eta_J}\right), \quad P_{\text{dir}}^{(S)} = w E_0 \rho_S \eta^3 (\eta^3 - \eta_c^3) \Theta(\eta - \eta_c), \quad \eta \equiv \frac{\rho \pi \sigma^2}{4}.$$

In Eq. (S75),  $\eta_c$  is the critical packing fraction for the WCA solid, while  $\eta_J$  is the jamming packing fraction of the active phase. The physical interpretation behind our ansatz is the following. The first term  $P_{\text{dir}}^{(R)}$  encompasses the interactions of rolling particles  $\rho_R$  with all other particles via the exponential term, responsible for the pressure increase due to jamming. Then, the second term  $P_{\text{dir}}^{(S)}$  contains the interaction of standing particles  $\rho_S$  with all their neighbours, which again gives rise to a sharp increase of the pressure at large densities. Once again, we stress that  $\rho_R, \rho_S$  are enslaved to  $\rho$  through the relaxation equation Eq. (3) of the main text, which means that  $P_{\text{dir}}$  is eventually a function of the total density  $\rho$  only.

### E. Numerical tests

To test the expression of the generalized active pressure Eq. (S53) and direct pressure Eq. (S75), we compare them against microscopic simulations of well-mixed systems of rolling and standing particles. To this purpose, we simulate our model in the weakly-arresting regime  $\alpha_0 < \beta_0$ , where the well-mixed homogeneous configuration is observed to be stable. In SI Fig. 3 we report the comparison between our numerical measurements and the predicted curves (S53) and (S75). We observe a good agreement between the two without any fitting parameter, suggesting that our equations can be used to model the generalized pressure in our system.

### F. From the generalized pressure to the binodal densities

Thanks to the procedure detailed in the previous sections, we now have a closed formula for  $\tilde{P}(\rho)$ :

$$\tilde{P}(\rho) = \underbrace{P_{\text{dir}}(\rho) + P_{\text{act}}(\rho)}_{P(\rho)} + \int^\rho \frac{\alpha'(s)}{D_r + \alpha(s)} P_{\text{act}}(s) ds. \quad (\text{S76})$$

where  $P_{\text{act}}$  and  $P_{\text{dir}}$  are respectively given by Eq. (S53) and Eq. (S75). The generalized free energy density  $g$  can then be reconstructed via Eq. (S60), which we recall here:

$$g(\rho) = \rho \int^\rho \frac{\tilde{P}(s)}{s^2} ds, \quad (\text{S77})$$

while the associated generalized chemical potential  $\mu \equiv g'(\rho)$  reads:

$$\mu(\rho) = \frac{\tilde{P}(\rho)}{\rho} + \int^\rho \frac{\tilde{P}(s)}{s^2} ds. \quad (\text{S78})$$

The coexisting binodals  $(\rho_L, \rho_A)$  are finally obtained via a common-tangent construction on  $g$ , which corresponds to solving numerically:

$$\begin{cases} \mu(\rho_L) = \mu(\rho_A) \\ P(\rho_L) = P(\rho_A) \end{cases}. \quad (\text{S79})$$

## VI. MECHANICAL PRESSURE IN QUINCKE RODS

In this section, we relate the bulk pressures for the liquid and arrested phases to the pressures they exert on a confining wall, as reported in Fig. 6b of the main text. To this end, we follow Ref. [3] and compute the mechanical pressure exerted on an external confining wall.

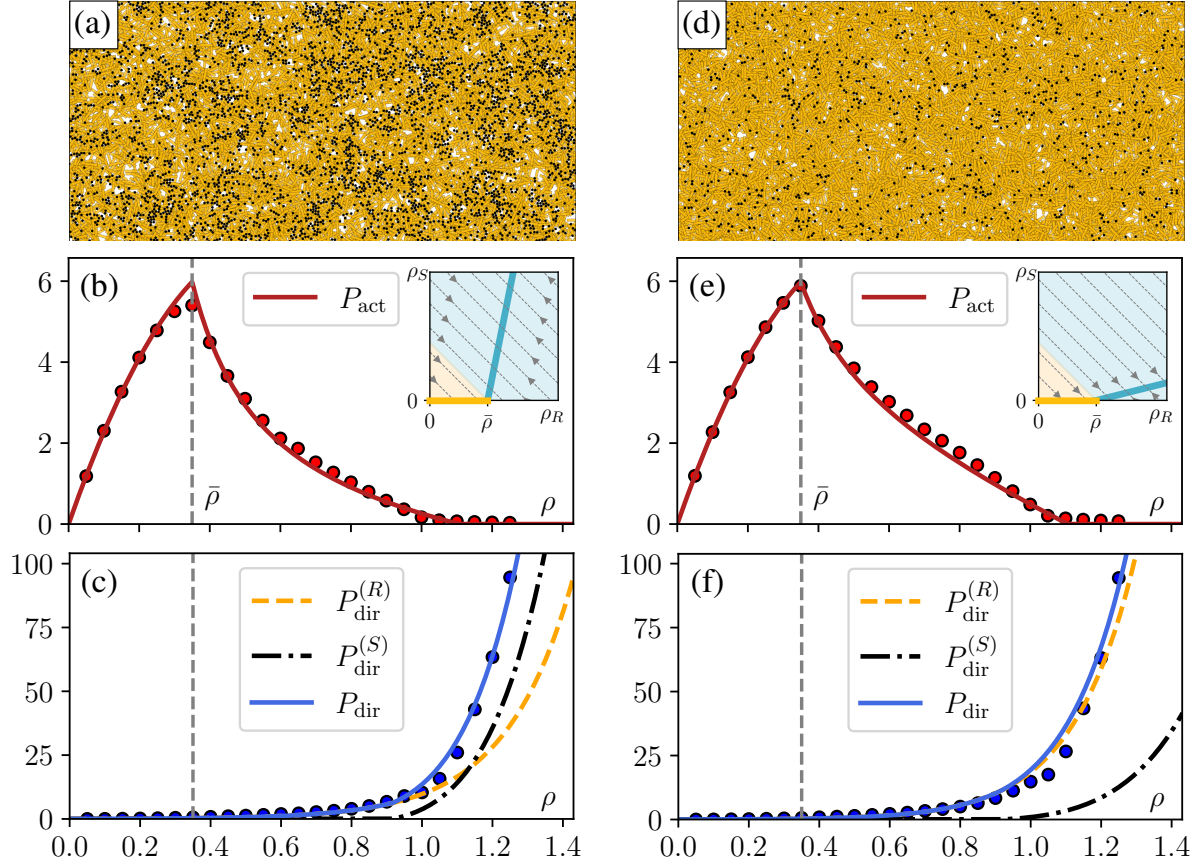

SI FIG. 3. **Direct and active pressures in a well-mixed system of rolling and standing particles.** Pressure measurements in a well-mixed system. Each column corresponds to a different value of  $\beta_0$ . (a, d) Snapshots of simulations in the well-mixed regime at a density  $\rho_0 = 0.6$ . (b, e) Active pressure  $P_{\text{act}}$ : comparison between numerical measurements and theoretical curves via Eq. (S53). The inset shows the mean-field relaxation dynamics in the  $(\rho_R, \rho_S)$ -space. (c, f) Direct pressure  $P_{\text{dir}}$ : comparison between numerical measurements and theoretical predictions via Eq. (S75). The curves  $P_{\text{dir}}^{(R)}$ ,  $P_{\text{dir}}^{(S)}$  represent the contributions of rolling and standing particles to  $P_{\text{dir}}$ , respectively.  $P_{\text{dir}}$  is defined as the sum of these two contributions. Note that the free parameters  $\rho_J, \xi, z$  of the theory for both  $P_{\text{act}}$  and  $P_{\text{dir}}$  have been obtained from previous simulations of PFAPs in the absence of switching transitions. Common parameters to all panels:  $L_x = 200, L_y = 100, D_r = 2, v_0 = 10, \alpha_0 = 10, \bar{\rho} = 0.35, \ell_r = 5, \sigma = 1, \mu = 1, E_0 = 1$ . In panels a-c,  $\beta_0 = 12$ ; in panels d-f,  $\beta_0 = 50$ .

We take periodic boundary conditions along  $y$ , and consider two confining walls located at  $x = 0$  and  $x = L$  modelled by external repulsive potentials  $U_{\text{ext}}(x)$  that are non-zero only close to the walls. The mechanical pressure  $P_{\text{mech}}$  on a wall is then defined as the force per unit length that the system exerts on the walls. By Newton's third law, for the wall located at  $x = L$ , this is equal to:

$$P_{\text{mech}} = \int_{\Lambda}^{\infty} dx U'_{\text{ext}}(x) \rho(x), \quad (\text{S80})$$

where  $x = \Lambda$  denotes any plane in the bulk phase next to the wall, and  $\rho(x)$  is the average density profile at steady state.

We start by writing the dynamics of the different harmonics in the presence of the walls:

$$\partial_t \hat{\rho}_S = -\nabla_{\mathbf{r}} \cdot \left[ -\mu \nabla_{\mathbf{r}} U_{\text{ext}} \rho_S + \mu \left\langle \int d^2 \mathbf{r}' \mathbf{f}(|\mathbf{r} - \mathbf{r}'|) \hat{\rho}(\mathbf{r}') \hat{\rho}_S(\mathbf{r}) \right\rangle \right] + \alpha \rho_R - \beta \rho_S, \quad (\text{S81})$$

$$\partial_t \psi_R = -\nabla_{\mathbf{r}} \cdot \left[ v_0 \mathbf{u} \psi_R - \mu \nabla_{\mathbf{r}} U_{\text{ext}} \psi_R + \mu \left\langle \int d^2 \mathbf{r}' \mathbf{f}(|\mathbf{r} - \mathbf{r}'|) \hat{\rho}(\mathbf{r}') \hat{\psi}_R(\mathbf{r}) \right\rangle \right] + \nabla_{\theta}^2 [D_r \psi_R] - \alpha \psi_R + \frac{\beta}{2\pi} \rho_S, \quad (\text{S82})$$

$$\partial_t \rho_R = -\nabla_{\mathbf{r}} \cdot \left[ v_0 \mathbf{m}_R - \mu \nabla_{\mathbf{r}} U_{\text{ext}} \rho_R + \mu \left\langle \int d^2 \mathbf{r}' \mathbf{f}(|\mathbf{r} - \mathbf{r}'|) \hat{\rho}(\mathbf{r}') \hat{\rho}_R(\mathbf{r}) \right\rangle \right] - \alpha \rho_R + \beta \rho_S. \quad (\text{S83})$$

Summing Eqs. (S81) and (S83) we obtain the dynamics of the total density, which has the form of a continuity equation:  $\partial_t \rho = -\nabla_{\mathbf{r}} \cdot \mathbf{J}$ . In the steady state, the system is translationally invariant along  $y$  and the associated mass current  $J_x$  along  $x$  is zero, due to the presence of the walls. Hence:

$$0 = v_0 m_{R,x} - \mu U'_{\text{ext}}(x) \rho + \mu \partial_x \sigma_{\text{IK},xx}. \quad (\text{S84})$$

We can thus express the mechanical pressure by isolating  $U'_{\text{ext}} \rho$  in Eq. (S84) and integrating over  $x$ :

$$\begin{aligned} P_{\text{mech}} &= \frac{v_0}{\mu} \int_{\Lambda}^{\infty} m_{R,x} dx + \int_{\Lambda}^{\infty} \partial_x \sigma_{\text{IK},xx} dx \\ &= \frac{v_0}{\mu} \int_{\Lambda}^{\infty} m_{R,x} dx + P_{\text{dir}}(\Lambda), \end{aligned} \quad (\text{S85})$$

where we used the definition of direct pressure  $P_{\text{dir}} = -\sigma_{\text{IK},xx}$  and the fact that  $P_{\text{dir}}(\infty) = 0$ .

We now need to express  $m_{R,x}$  in Eq. (S85). Multiplying the dynamics (S82) of  $\psi_R$  by  $\cos \theta$  and integrating over  $\theta$ , we find the expression of  $m_{R,x}$  at steady state:

$$m_{R,x} = -\frac{1}{D_r + \alpha(\tilde{\rho})} \partial_x \left[ v_0 \left( \frac{\rho_R}{2} + Q_{R,xx} \right) - \mu U'_{\text{ext}}(x) m_{R,x} + \mu \mathcal{I}_{m,xx} \right]. \quad (\text{S86})$$

where:

$$\mathcal{I}_{m,xx} \equiv \left\langle \int d^d \mathbf{r}' f_x(|\mathbf{r} - \mathbf{r}'|) \hat{\rho}(\mathbf{r}') m_{R,x}(\mathbf{r}) \right\rangle. \quad (\text{S87})$$

All in all, inserting Eq. (S86) in the expression (S85) for the mechanical pressure  $P_{\text{mech}}$  we obtain:

$$P_{\text{mech}} = P_{\text{dir}}(\Lambda) - \frac{v_0}{\mu} \int_{\Lambda}^{\infty} \frac{1}{D_r + \alpha(\rho(x))} \partial_x \left[ v_0 \left( \frac{\rho_R}{2} + Q_{R,xx} \right) - \mu U'_{\text{ext}}(x) m_{R,x} + \mu \mathcal{I}_{m,xx} \right] dx. \quad (\text{S88})$$

Integrating by parts we have:

$$P_{\text{mech}} = \underbrace{P_{\text{dir}}(\Lambda) + P_{\text{act}}(\Lambda)}_{P(\Lambda)} + \int_{\Lambda}^{\infty} dx \tilde{f}_x(x), \quad (\text{S89})$$

where we defined the bulk active pressure  $P_{\text{act}}$  as:

$$P_{\text{act}} = \frac{v_0}{\mu [D_r + \alpha]} \left[ v_0 \left( \frac{\rho_R}{2} + Q_{R,xx} \right) + \mu \mathcal{I}_{m,xx} \right], \quad (\text{S90})$$

the total bulk pressure  $P = P_{\text{act}} + P_{\text{dir}}$ , and the equation-of-state-breaking (EOS-breaking) term  $\tilde{f}_x$  as:

$$\tilde{f}_x(x) = \left[ \frac{v_0^2}{\mu} \left( \frac{\rho_R}{2} + Q_{R,xx} \right) + v_0 \mathcal{I}_{m,xx} - v_0 U'_{\text{ext}} m_{R,x} \right] \partial_x \left[ \frac{1}{D_r + \alpha(x)} \right]. \quad (\text{S91})$$

Due to the presence of the EOS-breaking terms, the mechanical pressure (S89) cannot be generically expressed as a function of bulk properties only. Despite this, there are some limit cases in which an EOS is actually recovered, as highlighted in Sec. III.D of the main text. When the standing rate  $\alpha$  is constant, the mechanical pressure is simply given by  $P_{\text{mech}} = P$  and the system admits an equation of state. This clearly applies to the active liquid phase where  $\alpha = 0$  everywhere. The active pressure, given by Eq. (S90), is a function of the harmonics of rolling particles only, and the mass of the associated polar field is renormalized as  $D_r \rightarrow D_r + \alpha$ . The presence of a finite arrest rate  $\alpha$  thus plays two roles: it controls the persistence time, and hence the relaxation rate of the polar field; and it controls the density of rolling particles, together with the associated harmonics  $\mathbf{m}_R, \mathbf{Q}_R$ . All in all, these two phenomena conspire to decreasing the active pressure.

In the arrested phase, instead, all active contributions and the EOS-breaking terms in Eq. (S89) vanish, and the

mechanical pressure  $P_{\text{mech}}$  is simply given by the direct contribution  $P_{\text{dir}}$ .

Let us finally consider what happens at the interface between an arrested solid phase and an active liquid of rolling particles. Following the argument above, each phase separately satisfies an EOS, but their bulk pressures are unequal due to the EOS-breaking term at the interface: when active particles roll towards the dense phase, they tend to switch to the standing state and thus exert collectively a mechanical force onto the arrested solid that is lower than what their bulk pressure suggest. Our simulations indeed confirm that the pressure in the solid phase is lower than in the liquid phase, and that both are equal to the force densities exerted on confining walls, as detailed in Fig. 6.

## VII. NUMERICAL DETAILS

Here we provide all details required to reproduce our numerical measurements, together with the list of parameters for the figures of the main text.

### A. Figure parameters

- Fig. 3.  $v_0 = 10, \alpha_0 = 20, \beta_0 = 10, D_r = 2, \ell_r = 5, \rho_0 = \bar{\rho} = 0.20$ , system size  $150 \times 150$  with periodic boundary conditions.
- Fig. 4. In all panels,  $\alpha_0 = 20, \beta_0 = 10, D_r = 2, \ell_r = 5, \sigma = 1, \mu = 1, E_0 = 1$ , system size  $200 \times 200$  with periodic boundary conditions. In (a-e),  $\bar{\rho} = 0.35, v_0 = 10$ . In (b),  $\rho_0 = 0.25$ . In (c),  $\rho_0 = 0.45$ . In (f-g),  $\rho_0 = 0.20, \bar{\rho}$  varies between 0.1 and 0.4, while  $v_0$  varies between 2 and 8.
- Fig. 5. In all panels,  $v_0 = 10, \alpha_0 = 20, \beta_0 = 10, D_r = 2, \ell_r = 5, \sigma = 1, \mu = 1, E_0 = 1$ . System size in (a):  $200 \times 200$  with periodic boundary conditions both in  $x$  and  $y$ . Numerical data in (b-d) are obtained from simulations in a  $300 \times 100$  domain with periodic boundary conditions along  $y$ . Along  $x$ , particles are confined by a soft harmonic wall of stiffness  $k = 3$ . They start to interact with the wall at a distance  $\delta = 5$  from the boundaries of the simulation domain. In (c, d),  $\bar{\rho} = 0.35$ .

### B. Bulk pressure measurements

To measure the bulk pressure in simulations, we first define a bulk region  $\mathcal{B} \equiv [x_-, x_+] \times [0, L_y]$  where we measure the pressure, and that we choose sufficiently far from walls and interfaces. The area of this region is denoted  $A_{\text{bulk}}$ . In simulations with two coexisting phases, such as in Fig. 6 of the main text, we measure the pressure in two bulk regions  $\mathcal{B}_1, \mathcal{B}_2$ , located inside each phase.

The active pressure  $P_{\text{act}}$  at time  $t$  is computed as:

$$P_{\text{act}}(t) = \frac{v_0}{2\mu[D_r + \alpha(\rho)]} \frac{1}{A_{\text{bulk}}} \left\{ \sum_{j \in \mathcal{B}}^{(R)} \dot{\mathbf{r}}_j(t) \cdot \mathbf{u}_j(t) + \sum_{j \in \mathcal{B}}^{(R)} [2 \cos^2 \theta_j(t) - 1] \right\}, \quad (\text{S92})$$

where the sum  $\sum^{(R)}$  runs over particles in the rolling state only. The density  $\rho$  is defined as the total number of particles in  $\mathcal{B}$  divided by  $A_{\text{bulk}}$ . The final value of the active pressure is obtained by averaging over measurements at different times:  $P_{\text{act}} = \frac{1}{K} \sum_{i=1}^K P_{\text{act}}(t_i)$ .

We now describe how we measure the Irving-Kirkwood or direct pressure in bulk phases. At time each sampling time  $t$  we compute:

$$P_{\text{dir}}(t) = \frac{1}{A_{\text{bulk}}} \sum_{x_i > x_j} f_{ij,x} [\mathbf{r}_i(t) - \mathbf{r}_j(t)] [x_i(t) - x_j(t)]. \quad (\text{S93})$$

where  $\mathbf{f}_{ij}$  is the force that particle  $i$  exerts on particle  $j$ . Importantly, when using this formula, one has to be careful when particles are close to the boundaries,  $x_-$  and  $x_+$ . More specifically:

- If both  $x_i, x_j \in \mathcal{B}$ , their contribution is given by  $f_{ij,x}(\mathbf{r}_i - \mathbf{r}_j)(x_i - x_j)$ .
- If  $x_i \in \mathcal{B}$  but  $x_j < x_-$ , their contribution to Eq. (S93) is corrected into  $f_{ij,x}(\mathbf{r}_i - \mathbf{r}_j)(x_i - x_-)$ .
- If  $x_j \in \mathcal{B}$  but  $x_i > x_+$ , their contribution to Eq. (S93) is corrected into  $f_{ij,x}(\mathbf{r}_i - \mathbf{r}_j)(x_+ - x_j)$ .



As done for the active pressure, we measure the direct pressure  $P_{\text{dir}}(t)$  at different times  $t$  using Eq. (S93) and average over time.

### C. Pressure measurements in the presence of a wall

To measure the mechanical pressure exerted on a confining wall, we simulate our system with periodic boundary conditions along  $y$ . To confine the system along  $x$ , we add two confining harmonic walls located at  $x = 0$  and  $x = L_x$ . Close to the left wall, a particle with position  $x$  is subjected to a harmonic potential  $V(x) = k(x - \delta)^2 \Theta(\delta - x)$ , where  $k$  is the wall stiffness and  $\delta$  is the cutoff distance at which particles start to interact with the wall. At the left wall, particles experience a confining harmonic force with same cutoff distance  $\delta$  and stiffness  $k$ . Every  $dt_{\text{meas}}$ , we measure the total pressure on a single wall as:

$$P_{\text{wall}}(t) = \frac{1}{L_y} \sum_i V'(x_i) \quad (\text{S94})$$

where the sum runs over the particles  $i$  that are close (within a distance  $\delta$ ) to the wall. The final value of the wall pressure is obtained by averaging over the different time steps.

### D. Coarsening

To characterize the coarsening dynamics in simulations, we first measure the time-dependent structure factor  $S(k, t)$  as follows. At a given time  $t$ , we create a  $2M \times M$  meshgrid of wave-vectors:  $k_x \in \frac{2\pi}{L} \{-M, \dots, M-1\}$ ,  $k_y \in \frac{2\pi}{L} \{0, \dots, M-1\}$ , where we set  $M = 32$ . For each wave-vector  $\mathbf{k} = (k_x, k_y)$  we compute the Fourier transform of the density field directly from the particles positions  $\{\mathbf{r}_i\}_{i=1}^N$ :

$$\hat{\rho}_{\mathbf{k}}(t) = \sum_{i=1}^N e^{-i\mathbf{k} \cdot \mathbf{r}_i(t)}, \quad (\text{S95})$$

and  $S(\mathbf{k}, t) \equiv |\hat{\rho}_{\mathbf{k}}(t)|^2 / N$ . Since the system is isotropic, we introduce  $S(k_n, t)$  as the average of  $S(\mathbf{k}, t)$  over all boxes within an annulus of radius  $k$ :  $\frac{2\pi}{L}n < k < \frac{2\pi}{L}(n+1)$ ,  $n \in \mathbb{N}$ .

We then compute the first moment of  $S(k, t)$  as:

$$\langle k(t) \rangle \equiv \frac{\int_0^{k_{\text{max}}} k S(k, t) dk}{\int_0^{k_{\text{max}}} S(k, t) dk}, \quad (\text{S96})$$

where  $k_{\text{max}}$  is the largest wave-vector that we sample in our simulations. The domain size is then estimated as  $R(t) \equiv 2\pi \langle k(t) \rangle^{-1}$ .

For different values of  $\rho_0$ , we fit the curve  $R(t)$  with a power law  $R(t; K, t_0) = K(t - t_0)^{1/3}$ , where  $K$  and  $t_0$  are free parameters. The curves for  $R/K$  as a function of  $(t - t_0)^{1/3}$  are shown to collapse well onto the same curve with slope 1.

### E. Area fraction

To estimate  $\Phi_A(\rho_0)$ , for a given value of the density  $\rho_0$ , we run  $M = 10$  simulations with different seeds for the random number generator. For each simulation  $k \in \{1, \dots, M\}$ , we compute the corresponding static area fraction  $\Phi_A^{(k)}$ , then we average over all  $M$  realizations to obtain the final value of  $\Phi_A(\rho_0)$ .

For the  $k$ -th realization, we determine  $\Phi_A^{(k)}$  as follows. At every instant of time we divide the simulation domain in squared pixels of linear size  $dx = 2\ell_r$ . For each pixel  $(i, j)$ , we compute the corresponding fraction  $f_A(i, j)$  of static particles. If  $f_A(i, j) > 80\%$ , then we say that the pixel  $(i, j)$  is a static pixel. The ratio between the number of static pixels over the total number of pixels gives us the area fraction  $\Phi_A^{(k)}(t)$ . Averaging over time samples of  $\Phi_A^{(k)}(t)$  at steady state finally provides us with the value of the static area fraction for the  $k$ -th simulation. Note that, in simulations with an arrested absorbing state, the area fraction is only measured in the last snapshot.

## F. Binodals

To measure the binodal densities in phase-separated systems, we divide the system in squared boxes of linear size  $2\ell_r$ . We then measure the density in each box and build the density histogram at a given time  $t$ . By averaging over time, we finally obtain the time-averaged density histogram for a given simulation. By fitting its peaks against two gaussians, we determine the densities of the coexisting phases. In simulations with an arrested absorbing state, we only measure the density histogram in the last snapshot.

## G. Hysteresis

Hysteresis cycles are performed by varying the arresting density  $\bar{\rho}$  and the self-propulsion speed  $v_0$  over time via a sawtooth protocol with period  $T$ .  $\bar{\rho}$  varies between a minimal value  $\bar{\rho}_{\min}$  and a maximal value  $\bar{\rho}_{\max}$ , as represented in Fig. 5g of the main text. At the same time,  $v_0$  varies between  $v_{\min}$  and  $v_{\max}$  in phase with  $\bar{\rho}(t)$ .

## VIII. CAPTIONS FOR SUPPLEMENTARY MOVIES

- **Caption for Movie 1.** Isotropic active liquid of colloidal rods (fluorescence imaging).  $3.7\ \mu\text{m}$ -long SU8 collidal rods motorized by the Quincke electroration mechanism. The rods form an isotropic active liquid. Fluorescence image (Only 25% of the rods are dyed).  $\rho_0 = 0.12\ \mu\text{m}^{-2}$ ,  $V = 210\ \text{V}$ .
- **Caption for Movie 2.** Isotropic active liquid of colloidal rods (bright field imaging).  $3.7\ \mu\text{m}$ -long SU8 collidal rods motorized by the Quincke electroration mechanism. The rods form an isotropic active liquid. Bright field image.  $\rho_0 = 0.12\ \mu\text{m}^{-2}$ ,  $V = 150\ \text{V}$ .
- **Caption for Movie 3.** No coexistence between the rolling and standing states in dilute systems for 3D printed Quincke rollers. The rollers are cylindrical rods of length 1 mm and width 0.17 mm motorized by the Quincke. We print the rods with a Formlabs Form 3 3D printer. We do not observe any rods in the standing state. They are either at rest at low  $E$ , or steadily roll.  $V = 4000\ \text{V}$ .
- **Caption for Movie 4.** Nucleation of the arrested phase. Nucleation and growth of an arrested phase in an active liquid. Bright field images.  $\rho_0 = 0.15\ \mu\text{m}^{-2}$ ,  $V = 109\ \text{V}$ .
- **Caption for Movie 5.** Particle exchange at the interface between the arrested and liquid phases. Fluorescence images of a static cluster that coexists with an active liquid phase. At the interface rods change their configuration to arrest or resume their propulsion.  $\rho_0 = 0.36\ \mu\text{m}^{-2}$ ,  $V = 270\ \text{V}$ .
- **Caption for Movie 6.** Absorbing phase transition for quorum-sensing active rods. In the absence of steric repulsion, quorum-sensing leads to an absorbing arrested phase (numerical simulations). Same parameters as in Fig. 4.
- **Caption for Movie 7.** Nucleation of the arrested phase in simulations. In the presence of both quorum sensing and pairwise steric repulsion we observe the nucleation of arrested clusters within an active liquid (numerical simulations). Same parameters as in Fig. 5b.
- **Caption for Movie 8.** Spinodal decomposition. In the presence of both quorum sensing and pairwise steric repulsion we observe typical spinodal-decomposition patterns at sufficiently large densities (numerical simulations). Same parameters as in Fig. 5c.
- **Caption for Movie 9.** Hysteresis loop in numerical simulations of Quincke rods with QS interactions and steric repulsion. We modulate the activity via a sawtooth protocol for  $\bar{\rho}$  and  $v_0$ . Same parameters as in Fig. 5g.
- **Caption for Movie 10.** Absorbing phase transition at high density in numerical simulations of Quincke rods with QS interactions and steric repulsion: At sufficiently high density, the homogeneous system can rapidly freeze into the arrested phase. Same parameters as in Fig. 5c except for  $\rho_0 = 0.80$ .
- **Caption for Movie 11.** Metastability of the arrested phase at high density in numerical simulations of Quincke rods with QS interactions and steric repulsion: The formation of active pockets can hinder the absorbing phase transition at high density for Quincke rods with QS interactions and steric repulsion (numerics). Same parameters as in Fig. 5c except for  $\rho_0 = 0.80$ .

- 
- [1] Note that, at this order  $\tilde{\rho} \simeq \rho$ ,  $\tilde{\rho}_R = \rho_R$ , and  $\tilde{\rho}_S \simeq \rho_S$ .
  - [2] J. Irving and J. G. Kirkwood, The statistical mechanical theory of transport processes. iv. the equations of hydrodynamics, The Journal of chemical physics **18**, 817 (1950).
  - [3] A. P. Solon, J. Stenhammar, R. Wittkowski, M. Kardar, Y. Kafri, M. E. Cates, and J. Tailleur, Pressure and phase equilibria in interacting active brownian spheres, Physical Review Letters **114**, 198301 (2015).
  - [4] A. P. Solon, J. Stenhammar, M. E. Cates, Y. Kafri, and J. Tailleur, Generalized thermodynamics of motility-induced phase separation: phase equilibria, laplace pressure, and change of ensembles, New Journal of Physics **20**, 075001 (2018).
  - [5] T. Speck, Coexistence of active brownian disks: Van der waals theory and analytical results, Physical Review E **103**, 012607 (2021).
  - [6] D. Martin, J. O'Byrne, M. E. Cates, É. Fodor, C. Nardini, J. Tailleur, and F. Van Wijland, Statistical mechanics of active ornstein-uhlenbeck particles, Physical Review E **103**, 032607 (2021).
